# Supplementary material for: Nonlinear chirped Doppler interferometry for \c{hi}(3) spectroscopy
Source: arXiv:2204.02259 source file (2022-04-05)
Supplement: Supplementary file 1 [file Supplemental.pdf]

# Nonlinear chirped Doppler interferometry for $\chi^{(3)}$ spectroscopy: supplemental document

This document provides supplementary information to "Nonlinear chirped Doppler interferometry for $\chi^{(3)}$ spectroscopy".

## 1. NUMERICAL MODEL

The spectrum and spectral phase of the pump and reference pulses are computed on a calculation grid of $N = 8192$ points spanning over a bandwidth of 1 PHz centered at the frequency of 291.3 THz (1030 nm). The matched time grid (via FFT) has a time step $\delta t = 5$ fs and a span of $N\delta t = 2.05$ ps, The input spectra are Gaussian spectra with a spectral width of 4.4 THz FWHM. Pump and probe pulses are equally chirped, with a chirp coefficient of $\varphi_{\mathrm{P}}^{(2)} = \varphi_{\mathrm{Pr}}^{(2)} = +5000$ fs $^2$. Reference pulse has a chirp coefficient of $\varphi_{\mathrm{R}}^{(2)} = \varphi_{\mathrm{Pr}}^{(2)} + \Delta\varphi_{\mathrm{RPr}}^{(2)}$, with either $\Delta\varphi_{\mathrm{RPr}}^{(2)} = +2000\,\mathrm{fs}^2$. The initial group delay between the probe and the reference pulses is $\tau_{\mathrm{Pr}}^{0}$=3 ps.

The time-dependent complex amplitude and intensity of the input pump/probe pulse are computed once for all via a discrete inverse Fourier transform (iFFT) and normalized so that the peak time intensity is equal to 1. The complex amplitude of the reference pulse is also computes once for all from the input spectrum and the phase coefficients given above.

The work flow for the numerical calculation of the spectral pattern (interferogram) between the probe and reference pulses is the following:

1. Shift the time intensity profile of the pump pulse by a time increment $\tau_{RPr} = -k\delta t$ where k is an integer
2. Multiply the latter by the maximum nonlinear phase shift $\phi_{\mathrm{XPM,\,max}}$ = 300 mrad
3. Take the complex exponential of the resulting product
4. Multiply by the complex amplitude of the initial pump pulse (ie unsifted). The pump and probe pulses are indeed assumed to have the same temporal properties
5. Compute the forward discrete Fourier transform (FFT) to get the complex amplitude of the probe pulse
6. Add the latter result to the complex amplitude of the reference pulse and compute the square modulus

The peak position is then extracted by the same routine as for the experimental data (described hereafter).

## 2. ANALYTICAL MODEL

An analytical model is proposed to illustrate the encoding of the Doppler shift of the probe pulse as a group delay change, when recombining the shifted signal with a chirped delayed local oscillator (reference). Here, we neglect two-beam coupling, i.e. pump and probe pulses are unchirped. XPM is modeled as a small spectral shift. The notations are simplified compared to the manuscript.

Let $E_{\mathrm{P}}(\omega)$, $E_{\mathrm{R}}(\omega)$ and $E_{\mathrm{Pr}}(\omega)$ be the complex spectral amplitudes of, respectively, the pump, reference and probe pulses. Their respective spectral phases are $\varphi_{\mathrm{P}}(\omega)$, $\varphi_{\mathrm{R}}(\omega)$, $\varphi_{\mathrm{Pr}}(\omega)$ with the convention $E_k(\omega) = |E_k(\omega)| \exp\left[-i\varphi_k(\omega)\right]$ where $k$ is the wave label. Spectral phases are hereafter assumed as purely quadratic, with chirp coefficients respectively labeled $\varphi_k^{(2)}$. The spectral phases thus write

$$\varphi_k(\omega) = \varphi_k(\omega_0) + \tau_k(\omega_0)(\omega - \omega_0) + \varphi_k^{(2)}(\omega - \omega_0)^2/2 \tag{S1}$$

where $\tau_k = \tau_k(\omega_0)$ stands for the group delay. For plane waves, the spectrum of the interference pattern between the reference and the probe fields is:

$$S(\omega) = |E_{\mathrm{R}}(\omega)|^2 + |E_{\mathrm{Pr}}(\omega)|^2 + 2\mathrm{Re}\left\{E_{\mathrm{R}}(\omega)E^*_{\mathrm{Pr}}(\omega)\mathrm{e}^{i\omega\tau_{RPr}}\right\} \tag{S2}$$

We define

$$\omega_0 = \int \omega|E_{\mathrm{P}}(\omega)|^2 d\omega \bigg/ \int |E_{\mathrm{P}}(\omega)|^2 d\omega$$

and

$$\Delta\omega^2 = \int (\omega-\omega_0)^2|E_{\mathrm{P}}(\omega)|^2 d\omega \bigg/ \int |E_{\mathrm{P}}(\omega)|^2 d\omega$$

as, respectively, the carrier angular frequency and the spectral bandwidth of the input pump pulse. The modulus of the spectral amplitude $|E_{\mathrm{P}}(\omega)|$ may be expressed as $|E_{\mathrm{P}}(\omega)| = |A_{\mathrm{P}}(\omega-\omega_0)|$ where $A_{\mathrm{P}}(\omega)$ is centered at $\omega = \omega_0$ in the sense that $\int w|A_{\mathrm{P}}(\omega-\omega_0)|^2 d\omega = 0$.

We assume the following:

- the spectrum of the input pulses is narrowband
- the probe pulse is a replica of the pump pulse
- the reference pulse is a time-delayed and chirped replica of the pump pulse with a group delay $\tau$ and a second-order phase coefficient $\varphi_2$
- the cross-phase modulation is modeled by a small spectral shift $\Omega \ll \Delta\omega$

These assumptions can be written as:

$$\begin{cases} \Delta\omega \ll \omega_0 & \text{(S3a)} \\ A_{\mathrm{P}}(\omega+\delta\omega) = A_{\mathrm{P}}(\omega-\delta\omega) & \text{(S3b)} \\ |E_{\mathrm{R}}(\omega)| = |E_{\mathrm{Pr}}(\omega)| = |E_{\mathrm{P}}(\omega)| = |E(\omega)| & \text{(S3c)} \\ \varphi_{\mathrm{R}}(\omega) = \varphi_{\mathrm{P}}(\omega) + \varphi_0 + (\omega-\omega_0)\tau + \dfrac{\varphi_2}{2}(\omega-\omega_0)^2 & \text{(S3d)} \\ E_{\mathrm{P}}(\omega) = E_{\mathrm{P}}(\omega+\Omega) \text{ with } \Omega \ll \Delta\omega & \text{(S3e)} \\ \varphi''_{\mathrm{P}}(\omega) = \varphi''_{\mathrm{P}}(\omega_0) & \text{(S3f)} \end{cases}$$

Let $\Delta\varphi(\omega) = \varphi_{\mathrm{R}}(\omega) - \varphi_{\mathrm{P}}(\omega)$ be the difference between the spectral phases of the reference and probe pulses. The cross-term of the Fourier-transform of $S(\omega) = S(\omega,\tau)$ along the $\omega$ coordinate is:

$$\hat{S}(t,\tau) = \int |E(\omega)||E(\omega+\Omega)|\mathrm{e}^{-i\Delta\varphi(\omega)}\mathrm{e}^{i\omega t}d\omega \tag{S4}$$

For $\Omega << \omega \simeq \omega_0$, the effect of the spectral shift can be approximated by:

$$|E(\omega+\Omega)| \simeq |E(\omega)| + \frac{\partial|E(\omega)|}{\partial\omega}\Omega \tag{S5}$$

which leads to:

$$\hat{S}(t,\tau) = \int |E(\omega)|^2\mathrm{e}^{-i\Delta\varphi(\omega)}\mathrm{e}^{i\omega t}d\omega + \Omega\int |E(\omega)|\frac{\partial|E(\omega)|}{\partial\omega}\mathrm{e}^{-i\Delta\varphi(\omega)}\mathrm{e}^{i\omega t}d\omega \tag{S6}$$

By integration by parts comes:

$$\hat{S}(t,\tau) = (1 - i\frac{\Omega t}{2})\int |E(\omega)|^2\mathrm{e}^{-i\Delta\varphi(\omega)}\mathrm{e}^{i\omega t}d\omega + i\frac{\Omega}{2}\int\frac{\partial\Delta\varphi}{\partial\omega}|E(\omega)|^2\mathrm{e}^{-i\Delta\varphi(\omega)}\mathrm{e}^{i\omega t}d\omega \tag{S7}$$

The phase difference $\Delta\varphi$ may be approximated to the first order in $\Omega$ by:

$$\Delta\varphi(\omega) \simeq \varphi_0 + (\omega-\omega_0)\tau + \varphi_2(\omega-\omega_0)^2/2 - \Omega\frac{\partial\varphi}{\partial\omega}$$

so that :

$$\frac{\partial \Delta\varphi}{\partial \omega} \simeq \tau + \varphi_2(\omega - \omega_0) - \Omega \frac{\partial^2 \varphi}{\partial \omega^2} \tag{S8}$$

where $\frac{\partial^2 \varphi}{\partial \omega^2}$ is a constant. Equation S7 may therefore by expanded as:

$$\hat{S}(t,\tau) = \left[1 - i\frac{\Omega(t-\tau)}{2}\right] \int |E(\omega)|^2 \mathrm{e}^{-i\Delta\varphi(\omega)} \mathrm{e}^{i\omega t} d\omega + i\frac{\Omega\varphi_2}{2} \int (\omega - \omega_0)|E(\omega)|^2 \mathrm{e}^{-i\Delta\varphi(\omega)} \mathrm{e}^{i\omega t} d\omega \tag{S9}$$

or, equivalently,

$$\hat{S}(t,\tau)\mathrm{e}^{(\varphi_0 + \omega_0 t)} \simeq \left[1 - i\frac{\Omega(t-\tau)}{2}\right] I(t - \tilde{\tau}) + \frac{\Omega\varphi_2}{2}\frac{\partial I}{\partial t}(t - \tilde{\tau}) \tag{S10}$$

where $I(t)$ is the Fourier-transform of $|A(\omega)|^2 \exp\left(-i\varphi_2\omega^2/2\right)$ and $\tilde{\tau} = \tau - \Omega\frac{\partial^2\varphi}{\partial\omega^2}$ is equal the group delay $\tau$ with a small correction in $\Omega$ when the input pulses are not limited by Fourier-transform. Note that $I(t)$ is, in principle, a complex-valued function that must be distinguished from the (real-valued) temporal profile. For the sake of the demonstration, since this correction does not depend on $\varphi_2$, we will assume $\tilde{\tau} = \tau$ in the following, which is equivalent to assume Fourier-transform-limited input pulses. However, this correction does not carried out in the final result. Let $\Delta\tau = t - \tau$. The modulus of the Fourier component at $t$ is, to the first order in $\Omega$:

$$|\hat{S}(t,\tau)| \simeq \left| I(\Delta\tau) - i\frac{\Omega}{2} I(\Delta\tau)\Delta\tau + \frac{\Omega\varphi_2}{2}\frac{\partial I(\Delta\tau)}{\partial t} \right| \tag{S11}$$

$$\simeq |I(\Delta\tau)| \left| 1 - i\frac{\Omega}{2}\Delta\tau + \frac{\Omega\varphi_2}{2}\frac{1}{I(\Delta\tau)}\frac{\partial I(\Delta\tau)}{\partial t} \right| \tag{S12}$$

$$\simeq |I(\Delta\tau)| + \frac{\Omega}{2}\varphi_2 |I(\Delta\tau)| \mathrm{Re}\left[\frac{1}{I(\Delta\tau)}\frac{\partial I(\Delta\tau)}{\partial t}\right] \tag{S13}$$

This result is general and applies to $|\hat{S}(t,\tau)|$ globally : the Fourier component at $t$ is the sum of $I(t-\tau)$ and a correction which scales with $\Omega$. We now focus on the shift of the maximum of $|\hat{S}(t,\tau)|$ as a function of $t$. The goal is to find the time $t_m$ for which $|\hat{S}(t,\tau)|$ admits a maximum. For a input spectrum $|A(\omega)|^2$ with an even parity about $\omega_0$ (such as a Gaussian spectrum centered at $\omega_0$), $I(t)$ is real-valued function which admits a maximum at $\Delta\tau_0 = 0$. For a non-symmetric spectral shape, the asymmetric part of $|A(\omega)|^2$ vanishes in the calculation of $I(t)$ so that only the symmetric part of the spectrum

$$A_{\mathrm{sym}}(\omega) = \left(|A(\omega)|^2 + |A(-\omega)|^2\right)/2$$

contributes to $I(t)$, which is, again, real-valued with a maximum at $t = 0$. It follows that $I(t)$ is actually real-valued with a maximum at time zero. $|\hat{S}(t,\tau)| = |\hat{S}(\delta t)|$ therefore admits a maximum in the vicinity $\Delta\tau \simeq 0$, or, equivalently, $t \simeq \tau$. It also follows that Eq. S11 can be approximated, to the first order in $\delta\tau$ by:

$$|\hat{S}(t \simeq \tau,\tau)| \simeq |I(\Delta\tau)| + \frac{\Omega}{2}\varphi_2 \left.\frac{\partial^2 I}{\partial t^2}\right|_{t=0} \Delta\tau \tag{S14}$$

For $\varphi_2 = 0$, $|\hat{S}(t \simeq \tau,\tau)| \simeq |I(\delta\tau|$ and the frequency shift $\Omega$ has no effect, ie the Fourier component has a maximum at $t = \tau$. For $\varphi_2 \neq 0$, the second term if the right-hand side of Eq. S14 tends to shift the maximum of the Fourier component along the $t$-axis by some quantity. For a general regular function $f(x)$ characterized by $f'(0) = 0$ and $f''(0) \neq 0$, $f(x) + \alpha x$ admits a maximum at $x_m$ where $x_m$ can be approximated, to the first order in $\alpha$, by:

$$x_m \simeq -\frac{\alpha}{f''(0)} \tag{S15}$$

This result, applied to formula S14 with $f(t) = |I(t)|$, leads to the following simple expression for shift :

$$\delta\tau = t_m - \tau \simeq -\frac{\Omega\varphi_2}{2} \tag{S16}$$

## 3. DATA ACQUISITION AND ANALYSIS

For each acquisition scan, $\tau_{\mathrm{PPr}}$ is continuously changed from -2.6 ps to 2.6 ps with 13 fs temporal resolution. The interference spectrum is acquired for each step, with a 2 ms integration time (400 spectra per scan). The probe-reference delay and relative chirp are measured before each acquisition, out of pump-probe temporal overlap.

The following work flow is used for each scan processing :

1. Fourier Transformation (FT) of each spectrum ;
2. Detection of the center of a Gaussian fit of the delay peak in the FT amplitude for each $\tau_{\mathrm{PPr}}$ step, with 0.3 fs numerical resolution;
3. Smoothing of the signal $\tau_{RPr} = f(\tau_{PPr})$ by moving average (window 5) to reduce the experimental noise;
4. Measurement of the contrast of the smoothed signal as: $\delta\tau = |\tau_{\mathrm{RPr,\,max}} - \tau_{\mathrm{RPr,\,min}}|$
5. Linear fitting of the smoothed signal between extrema of $\tau_{\mathrm{RPr}} = f(\tau_{\mathrm{PPr}})$ .
6. The relative phase between the two pulses as a function of pump probe delay can also be extracted, so as to compare our analysis with traditional nonlinear phase measurements. This is done by temporal filtering of the delay peak in the Fourier space and reverse Fourier Transform. The spectral dependence of the phase quantifies the relative chirp between probe and reference, for each acquisition.

We made 5 scans per sample for the validation of the method in bulk materials. Averaged values of $\alpha$ and $\delta\tau$ are normalized over the sample thickness and peak intensity. It is verified that with no nonlinear sample or if the pump is blocked no change in the spectrogram can be detected, ie the probe is too weak to be affected by self-phase modulation. The overall stability of $\tau_{\mathrm{RPr}}$ during the scan depends on the polarization configuration. For (i) and (ii) polarization configurations, the RMS noise is 0.3 fs; for (iii) and (iv) 3.5 fs.
